# Supplementary material for: PIM-QAT: Neural Network Quantization for Processing-In-Memory (PIM) Systems
Source: arXiv:2209.08617 source file (2022-09-18)
Supplement: Supplementary file 1 [file appendix.tex]

\setcounter{section}{0}
\setcounter{equation}{0}
\setcounter{figure}{0}
\setcounter{table}{0}

% \clearpage

% {\noindent\large\bf Appendix}

\input{tex_files/A1_proof_two_column}
\input{tex_files/A2_setting}
\input{tex_files/A3_scale_enlarging}
\input{tex_files/A4_running_stats_nonideality}
\input{tex_files/A5_scaling_factor}
\input{tex_files/A6_ablation}
\input{tex_files/A7_bn_calib}
